# Supplementary material for: Spiral bandwidth of four-wave mixing in Rb vapour
Source: arXiv:1805.08190 ancillary file (2018-11-28)
Supplement: Supplementary file 1 [file Supplementary.pdf]

**Supplementary Note 1: Experimental setup.** This section includes further details of the experimental setup. Due to the large detuning of the 780 nm laser from the $^{85}$Rb $5S_{1/2}$ $F = 3$ to $5P_{3/2}$ $F = 4$ transition we lock it using a dichroic atomic vapour laser lock (DAVLL)[1]. As this locking method is subject to slow drifts due to temperature changes affecting polarisation optics, we also monitor the detuning via a beat note with a separate locked 780 nm laser. The 776 nm laser is locked using two-photon spectroscopy in a heated rubidium cell (using counter propagating 780 nm and 776 nm beams) so that the pump fields are two-photon resonant with the $^{85}$Rb $5S_{1/2}$ $F = 3$ to $5D_{5/2}$ $F' = 5$ transition.

The holograms used to shaped the pump beams are detailed in[2–4]. In brief, the phase of the desired beam is combined with a phase grating, the depth of which is modulated by a function of the desired intensity profile. The required mode is generated in the first order diffracted from the phase grating, which is selected by an aperture in the Fourier plane of the SLM. Additional corrections can also be applied to either beam using the SLM, for example a spherical lens to adjust the axial position of the focus of the beam, or cylindrical lenses to reduce SLM astigmatism.

**Supplementary Note 2: Mode decomposition via Fourier analysis.** The mode decomposition method used is based on Fourier analysis of the interferogram formed at the output of a Dove prism interferometer. Each measurement requires three images: the intensity profile in interferometer arm A, $I_{\rm A}(r,\theta)$, the intensity profile in arm B, $I_{\rm B}(r,\theta)$, and the interferogram, $I_{\rm T}(r,\theta)$.

The electric field at the interferometer output for a pure LG mode is $E(r,\theta) = \sqrt{I_{\rm A}(r,\theta)}e^{-il\theta} + \sqrt{I_{\rm B}(r,\theta)}e^{il\theta+i\phi_p^l}$, where $\phi_p^l$ is the mode-dependent interferometer phase. The intensity at the interferometer output, or interferogram, is therefore:

$$I_{\rm T}(r,\theta) = I_{\rm A} + I_{\rm B} + 2\sqrt{I_{\rm A}I_{\rm B}}\cos(2l\theta + \phi_p^l) \tag{S1}$$

As noted in the main text, the total interferogram intensity for $l = 0$ modes is critically determined by the interferometer phase, $\phi_p^l$. In order to include these modes in the mode decomposition, and also correct for small discrepancies in 50:50 beam splitter transmission, we generate a corrected interferogram $I_{\rm C}(r,\theta)$:

$$I_{\rm C} = I_{\rm AB}(r)\left[1 + \frac{I_{\rm T}(r,\theta) - (I_{\rm A}(r,\theta) + I_{\rm B}(r,\theta))}{2\sqrt{I_{\rm A}(r,\theta)I_{\rm B}(r,\theta)}}\right], \tag{S2}$$

with $I_{\rm AB}(r) = \frac{1}{2}\left(\overline{I_{\rm A}}(r) + \overline{I_{\rm B}}(r)\right)$, where $\overline{I_{\rm A}}(r)$ and $\overline{I_{\rm B}}(r)$ are the average radial profile of $I_{\rm A}$ and $I_{\rm B}$ respectively. By comparison with Eq. S1, the square bracket term in Eq. S2 contains all of the interferogram's transverse phase information. The radial profile of the corrected interferogram, $I_{\rm C}$, is provided by the mean radial profile of the beam, $I_{\rm AB}(r)$, where the relative intensity of the modes has no dependence on the interferometer phase, $\phi_p^l$. We note that when $I_{\rm A}$ and $I_{\rm B}$ become small, intensity noise can cause $I_{\rm C}$ to become very large. To avoid this we do not perform the correction for interferogram pixels where either $I_{\rm A}$ or $I_{\rm B}$ fall below a threshold value.

The $\ell$-decomposition is found via Fourier analysis of the azimuthal profile of the corrected interferogram, $I_{\rm C}$. Before carrying out the $p$-decomposition, we chose the beam waist by performing a $p = 0$ one mode fit to the radial profile of $I_{\rm C}$, with the $\ell$ index of the mode used determined by the peak value from the $\ell$-decomposition. We then fit the $\ell$-components of the corrected interferogram, selected via two-dimensional Fourier filtering, with an incoherent sum of $p$-modes of the relevant $\ell$ index, and with the beam waist fixed at the value found from the initial one mode fit. Finally, the $\ell = 0$ modes are found from a final fit to the radial profile of $I_{\rm C}$, where the model consists of the $|\ell| > 0$ radial profile, multiplied by a single scale factor, plus an incoherent sum of $\ell = 0$ modes.

The two-dimensional Fourier filtering also allows some discrimination between noise and signal in the initial $\ell$-decomposition of the beam. If, after Fourier filtering, the resulting radial profile cannot be fit with $p$-modes of that particular $\ell$-value, then the profile must be due to noise in the Fourier transform, for example, due to misalignment of the interferometer. By discarding modes where the quality of the fit is very poor we can remove this noise from our measurement. We judge the goodness of fit based on the adjusted $R^2$[5], and reject modes where this value is less than 0.8.

**Supplementary Note 3: Full mode decomposition of the pump light.** Supplementary Fig. 1 a-d, e-h show the 776 nm and 780 nm pump beams, respectively, with (a,e) their profiles and interferograms and (b,f) their full $\ell$ and $p$-mode decomposition (cf. Fig. 2 main text). The analysis, detailed in the main text, was carried out for modes up to $\ell = 10$ and $p = 3$. Only modes up to $p = 2$ are shown here, all modes are in Dataset 1 (Ref.[6]). Most of the power is in the $p = 0$ modes (Supplementary Fig. 1 (c,g)), with the total power in modes with $p > 0$ less than 4% for all pump modes.

The relative power in the target mode is similar for both pump beams and reduces slightly as $\ell$ increases (Supplementary Fig. 1 (d,h)). There is also an increase in the error, which is the standard error over 5 measurements, as $\ell$ increases. The source of this noise is most likely due to air currents around the heated rubidium cell causing movement of the interferogram. This has a more pronounced effect at larger $\ell$ due to the narrower interference fringes. Other sources of error in the measurement include misalignment of the interferometer and small amounts of astigmatism introduced by the interferometer itself.

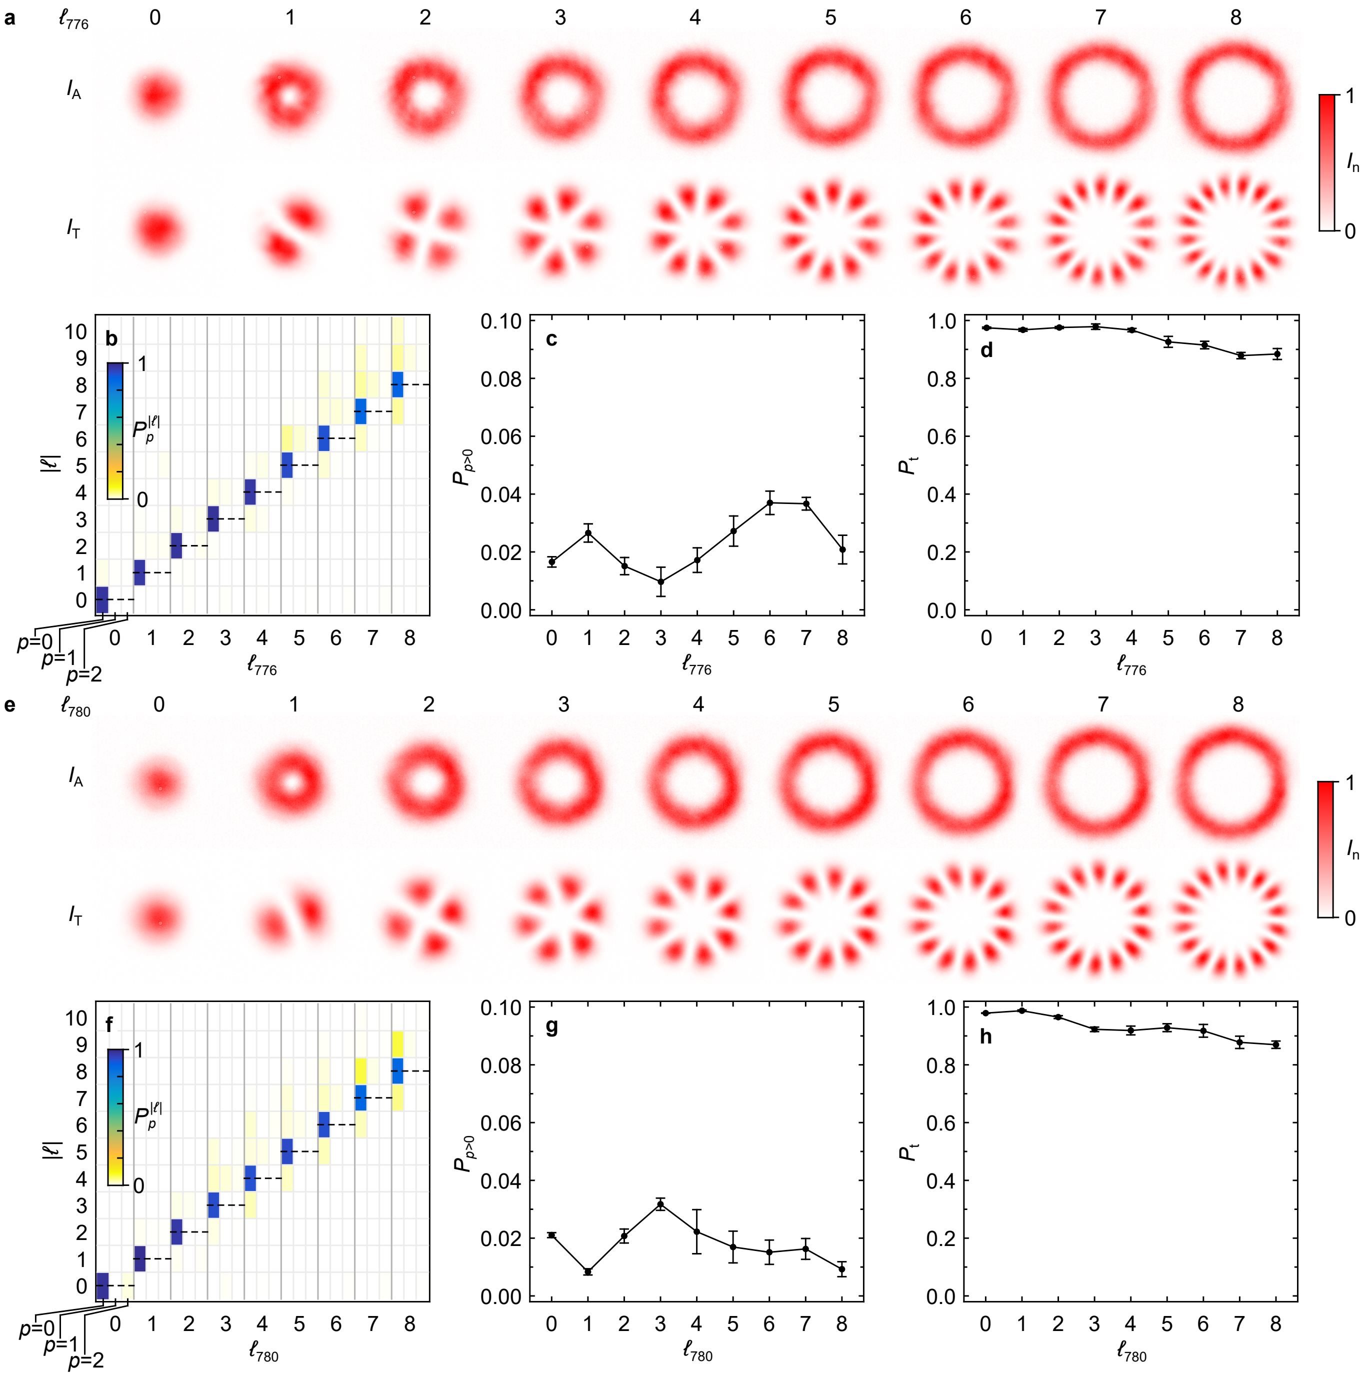


Supplementary Figure 1. Transverse mode analysis of the 776 nm (Fig. 3 main text) and 780 nm pump beams (a-d and e-h, respectively). (a,e) The beam profile $I_{\mathrm{A}}$ and interferogram $I_{\mathrm{T}}$ for each pump mode. (b,f) Full LG mode decomposition, in both $\ell$ and $p$, via Fourier analysis. The dashed lines mark the desired $\ell$ index in each case as a guide to the eye. (c,g) Relative power in the target mode. (d,h) Total relative power in modes with $p > 0$.

**Supplementary Note 4: Full mode decomposition of the 420nm light.** Supplementary Fig. 2 shows the generated 420 nm beam when only the 776 nm pump field carries OAM (a-f, Fig. 4 main text) and when both pump fields carry OAM (g-l, Fig. 5 main text), with beam profiles and interferomgrams (a,g), and the full $\ell$ and $p$-mode decomposition (b,h). The analysis was carried out for LG modes up to $p = 3$ (only modes up to $p = 2$ are shown, all modes are included in the dataset[6]).

We consider modes with $p \neq 0$ in our theoretical analysis, as in Ref. [7]. The predicted full mode decomposition of the 420 nm and 5.2 $\mu$m fields are shown in Supplementary Fig. 2 parts (c,i) and (d,j), respectively.

Plots of the total relative powers in the $p = 0, 1, 2$ and

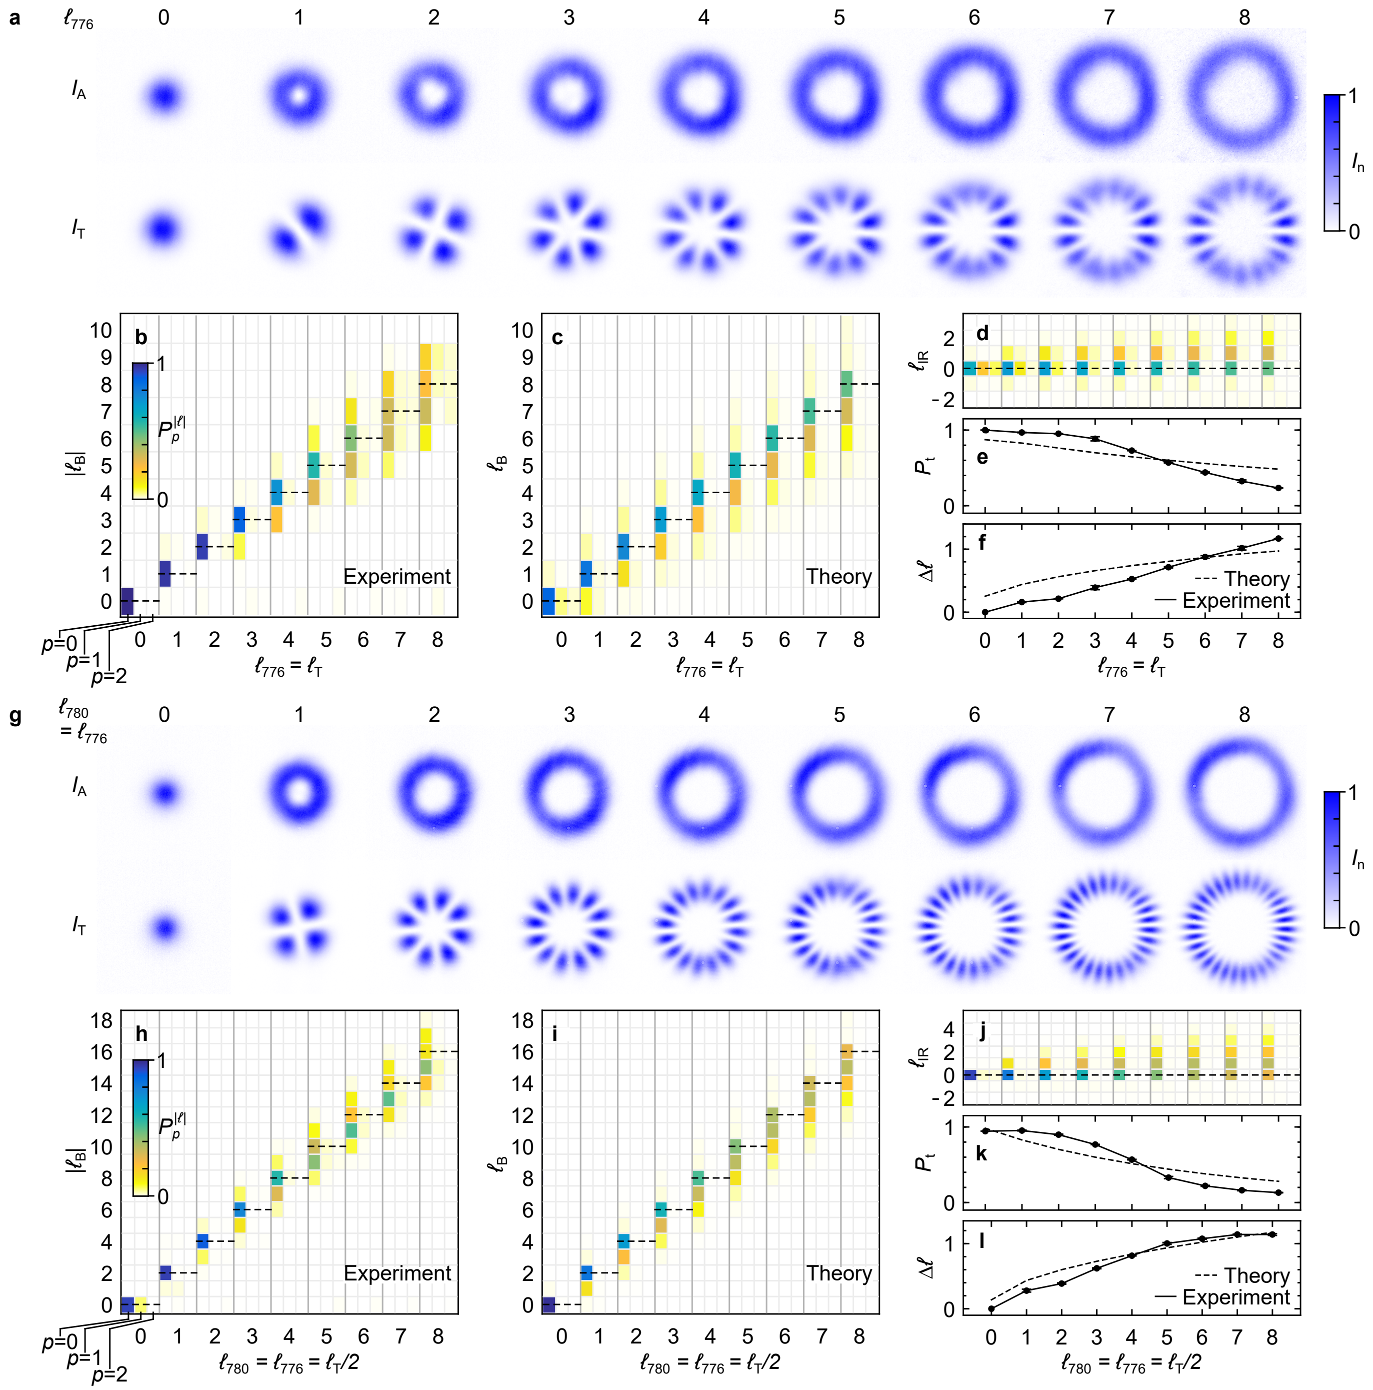


Supplementary Figure 2. Transverse mode analysis of the generated 420 nm light. Pump OAM carried only by the 776 nm beam (cf. Fig. 4 main text) and identical 780 nm and 776 nm pump OAM (cf. Fig. 5 main text) are shown in a-f and g-l, respectively. (a,g) The beam profile $I_A$ and interferogram $I_T$ for each pump mode. (b,h) Full LG mode decomposition, in both $\ell$ and $p$, via Fourier analysis. Full theoretical mode decomposition of the (c,i) 420 nm and (d,j) 5.2 $\mu$m fields. Relative power $P_t$ in the 420 nm mode $LG_0^{\ell_T}$ : $LG_0^{\ell_{776}}(e)$ or $LG_0^{\ell_{780}+\ell_{776}}$ (k). (f,l) Width of the 420 nm $p = 0$ $\ell$-decomposition indicating the available spiral bandwidth.

3 modes for each experiment in Supplementary Fig. 2 a-f and g-l are shown in the corresponding upper and lower Supplementary Fig. 3 a,b and c,d. As predicted by the theory, we observe the majority of the 420 nm light in $p = 0$ modes. Considering only the spatial intensity overlap of the fields this may be counterintuitive, as the $p > 0$ modes still have good spatial overlap with the pump beams. However, the differing Gouy phase of these

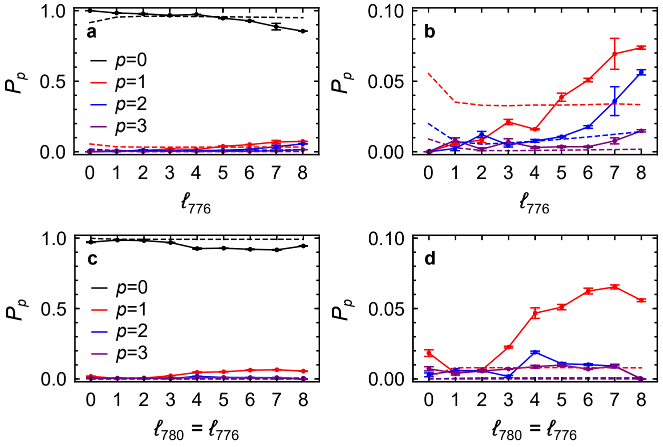


Supplementary Figure 3. The total relative power generated in the 420 nm $p = 0, 1, 2$ and 3 modes for the pump modes in Supplementary Fig. 2 a and b, are shown in a,b and c,d here, respectively. A zoomed version of a,c is shown in b,d highlighting the $p > 0$ modes more clearly. Solid lines: experiment, dashed lines: theory.

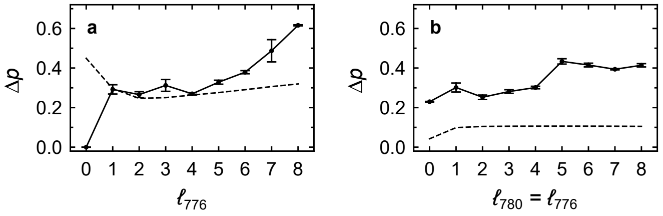


Supplementary Figure 4. The width of the 420 nm $p$-distribution for the results in Supplementary Fig. 2 a-f and g-l are correspondingly shown in a and b here. Solid lines: experiment, dashed lines: theory.

modes (as discussed in the main text) means that they are not well phase matched.

Gouy phase matching also affects the predicted 5.2 $\mu$m mode decomposition. The weaker Gouy phase matching when the pump beams are not focused to the same axial position results in significant power predicted in $p \neq 0$ modes in Supplementary Fig. 2 d. In contrast, in Supplementary Fig. 2 j, when the beams are focused to the same point and shaped into the same mode, the theory predicts much stronger Gouy phase matching and essentially all 5.2 $\mu$m light is expected to be in $p = 0$ modes.

For completeness, the measured and predicted width of the $p$-mode distribution for both experiments is shown in Supplementary Fig. 4. This gives an indication of the $p$-mode equivalent of the spiral bandwidth - the number of $p$-modes that could be entangled in the 5.2 $\mu$m and 420 nm two-photon state. When the pump OAM is supplied only by the 776 nm beam (Supplementary Fig. 4 (a)), there is some variation in the number of $p$-modes generated with pump $\ell$. There is less variation when the OAM is shared between the pump beams (Supplementary Fig. 4 (b)), both in the measurement and the theoretical prediction.

**Supplementary Note 5: Measured beam waists.** In the theoretical model presented in the main text, we assume that the waists obey the Boyd criterion (which was established for fundamental modes, focused to the same point). However, it is not obvious that this should also apply for higher order modes, especially when we separate the foci of the two pump beams. Indeed measurements of the 420 nm waist (Supplementary Fig. 5) show that in general the 420 nm light is not generated with the waist predicted by the Boyd criterion. This could explain the small discrepancies we seen between our results and theory. A more accurate prediction of the waists might be found by maximising the FWM signal in the theoretical model by varying each of the generated field waists.

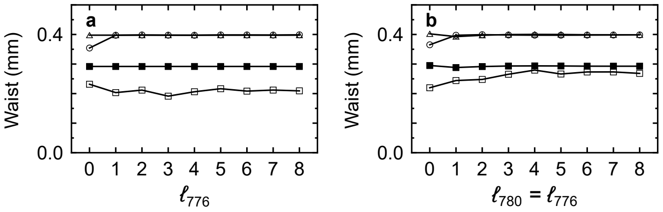


Supplementary Figure 5. 420 nm waist in the image plane after the rubidium cell (marked Im in Fig. 1 in the main text) for (a) OAM frequency conversion (Supplementary Fig. 2 a-f, Fig. 4 main text) and (b) OAM addition (Supplementary Fig. 2 g-l, Fig. 5 main text). Circles: 776 nm, Triangles: 780 nm, Empty squares: measured 420 nm, Filled squares: predicted 420 nm.

## Supplementary References

[1] Corwin, K. L., Lu, Z.-T., Hand, C. F., Epstein, R. J. & and Wieman, C. E. Frequency-stabilized diode laser with the Zeeman shift in an atomic vapor. *Appl. Opt.* **37**, 3295–3298 (1998).

[2] Clark, T. W., Offer, R. F., Franke-Arnold, S., Arnold, A. S. & Radwell, N. Comparison of beam generation techniques using a phase only spatial light modulator. *Opt. Express* **24**, 6249–6264 (2016).

[3] Radwell, N., Offer, R. F., Selyem, A. & Franke-Arnold, S. Optimisation of arbitrary light beam generation with spatial light modulators. *J. Opt.* **19**, 095605 (2017).

[4] Davis, J. A., Cottrell, D. M., Campos, J., Yzuel, M. J. & Moreno I. Encoding amplitude information onto phase-only filters. *Appl. Opt.* **38**, 5004–5013 (1999).

[5] Fahrmeir, L., Kneib, T., Lang, S. & Marx, B. *Regression models, methods and applications* (Springer, 2013) p. 147.

[6] Offer, R. F., Stulga, D., Riis, E., Franke-Arnold, S. & Arnold, A. S. Dataset DOI: 10.15129/96db0ebb-aace-494f-8e61-d4a064fcadbb (2018).

[7] Lanning, R. N. *et al.* Gaussian-beam-propagation theory for nonlinear optics involving an analytical treatment of orbital-angular-momentum transfer. *Phys. Rev. A* **96**, 013830 (2017).
